# Supplementary material for: High efficiency dark-to-bright exciton conversion in carbon nanotubes
Source: arXiv:1905.10043 ancillary file (2019-05-24)
Supplement: Supplementary file 1 [file ExcitonDynamicsSI.pdf]

# Supplemental Materials for "High efficiency dark-to-bright exciton conversion in carbon nanotubes"


A. Ishii,[1,2] H. Machiya,[1,3] and Y. K. Kato[1,2,*]

[1] *Nanoscale Quantum Photonics Laboratory, RIKEN Cluster for Pioneering Research, Saitama 351-0198, Japan*

[2] *Quantum Optoelectronics Research Team, RIKEN Center for Advanced Photonics, Saitama 351-0198, Japan*

[3] *Department of Electrical Engineering, The University of Tokyo, Tokyo 113-8656, Japan*

[*] Corresponding author. yuichiro.kato@riken.jp

## I. EXCITATION AND DETECTION WAVELENGTH DEPENDENCE OF PL DECAY DYNAMICS

We examine how excitation and emission wavelengths affect the PL decay curve using a 2.3-$\mu$m-long (9,7) CNT. For excitation, the $2u$ sub-peak at 890 nm can be selected in addition to the $E_{22}$ main peak at 785 nm as shown in the PLE map [Fig. S1(a)]. The emission spectrum has the $E_{11}$ main peak and a lower energy sub-peak from $K$-momentum excitons, which can be spectrally filtered by using an additional long-pass filter as shown in Fig. S1(b). We measure PL decay curves for different combinations of the excitation/emission wavelengths at a low excitation power. Figure S1(c) displays the normalized decay curves, showing almost perfect overlap. The independence on the detected emission peak implies that population equilibrium exists between bright and $K$-momentum states due to a very fast transition process, whereas the independence on the excitation wavelength indicates unchanged initial populations at bright and dark states. The result is consistent with a previous report [1], but is in contradiction with an expectation that initial populations should depend on the exciton relaxation path from the excited states. Understanding of scattering mechanisms in the relaxation pathways is nessesary to elucidate the initial population process.

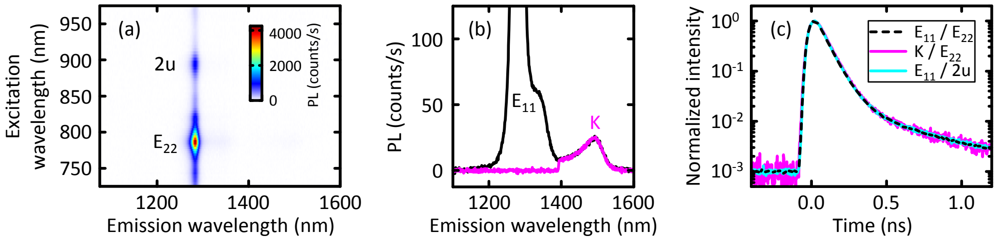


FIG. S1. (a) PLE map of a (9,7) CNTs. CW excitation with $P = 2$ $\mu$W is used. (b) PL spectra with (black) and without (magenta) a long-pass filter. CW excitation at $E_{22}$ resonance with $P = 2$ $\mu$W is used. (c) PL decay curves taken with different combinations of excitation and detection wavelengths. (black) $E_{22}$ excitation with $P = 5$ $\mu$W and $E_{11}$ detection. (magenta) $E_{22}$ excitation with $P = 5$ $\mu$W and $K$ detection. (cyan) $2u$ excitation with $P = 30$ $\mu$W and $E_{11}$ detection.

## II. EXCITATION POWER DEPENDENCE OF PL DECAY DYNAMICS

Next we change the excitation power to investigate the effects of exciton-exciton annihilation (EEA) process on the exciton dynamics. PL spectra are measured at $E_{22}$ excitation, and we observe sublinear increase of PL intensity as shown in Fig. S2(a), resulting from efficient EEA [2]. PL decay curves measured at different powers are shown in Fig. S2(b). The curve at the lowest power clearly shows two decay components, which reflects the exciton dynamics of bright and dark states as discussed in the main text. When the power is increased to the sublinear region, the fast component becomes faster, and an additional decay component in between the fast and slow decays emerges. The lifetime shortening of the fast component is a direct consequence of EEA involving bright excitons. The mechanism of the emergence of the intermediate decay component is not intuitive, but we speculate that EEA of dark excitons generate excited $E_{11}$ excitons, and their relaxation process may partially yield bright excitons. Such a process can enhance the apparent bright-dark transition rate and can explain the complex behavior of the power dependence.

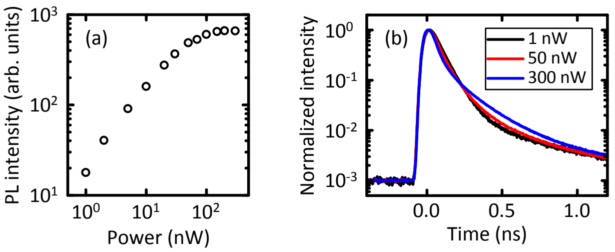


FIG. S2. (a) Excitation power dependence of PL intensity. (d) PL decay curves taken at different powers. In (a) and (b), the same (9,7) CNT used in Fig. S1 is measured with pulsed excitation at the $E_{22}$ wavelength.

## III. MOLECULAR DESORBED STATE AND ADSORBED STATE TRANSITION

In order to obtain the molecular desorbed state of CNTs, we heat the samples to 400°C in Ar gas with 3% $H_2$ for 20 min. Soon after taking out the sample, we take PLE maps for (9,7) and (10,5) CNTs as shown in Figs. S3(a) and (c), respectively. Both $E_{11}$ and $E_{22}$ wavelengths are blueshifted by the molecular desorption [3, 4], and the tubes return to the molecular adsorbed state [Figs. S3(b) and (d)] within 1–2 hours. In Fig. S3(e), the temporal evolution of PL emission wavelengths of the CNTs are shown, where distinct state transitions are observed. The (9,7) tube shows a shorter transition time compared to the smaller diameter (10,5) tube, and we find that the correlation between the diameter and the transition time is reproducible. A possible explanation is that the formation of stable layers of air molecules strongly depends on the surface area and curvature of CNTs.

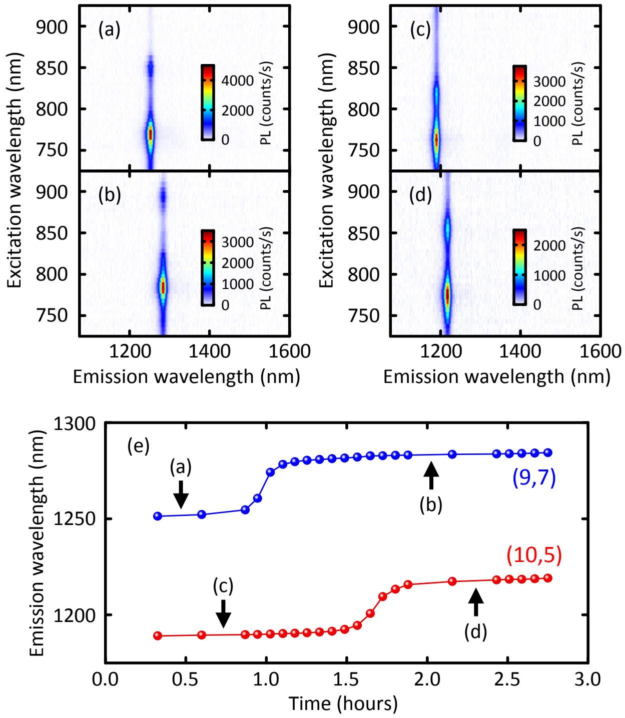


FIG. S3. (a) and (b) PLE maps of a (9,7) CNT at molecular desorbed and adsorbed states, respectively. (c) and (d) PLE maps of a (10,5) CNT at molecular desorbed and adsorbed states, respectively. (e) Time tracking plot of the emission wavelength after finishing the sample heating. Blue and red points show the data from the (9,7) and (10,5) CNTs, respectively. Time periods for the PLE measurements are indicated by arrows. $P = 2$ $\mu$W and laser polarization perpendicular to the trench direction are used in (a-e), and $\lambda_{ex} = 780$ nm is used in (e).

[1] T. Gokus, L. Cognet, J. G. Duque, M. Pasquali, A. Hartschuh, and B. Lounis, Mono- and biexponential luminescence decays of individual single-walled carbon nanotubes, J. Phys. Chem. C **114**, 14025 (2010).

[2] A. Ishii, M. Yoshida, and Y. K. Kato, Exciton diffusion, end quenching, and exciton-exciton annihilation in individual air-suspended carbon nanotubes, Phys. Rev. B **91**, 125427 (2015).

[3] J. Lefebvre and P. Finnie, Excited excitonic states in single-walled carbon nanotubes, Nano Lett. **8**, 1890 (2008).

[4] T. Uda, S. Tanaka, and Y. K. Kato, Molecular screening effects on exciton-carrier interactions in suspended carbon nanotubes, Appl. Phys. Lett. **113**, 121105 (2018).
